# Supplementary material for: Terahertz Spin-Light Coupling in Proximitized Dirac Materials
Source: arXiv:2410.21614 source file (2024-10-28)
Supplement: Supplementary file 1 [file Supplemental.pdf]

# Supplemental Material
# Terahertz Spin-Light Coupling in Proximitized Dirac Systems

Konstantin S. Denisov,[1,2,*] Igor V. Rozhansky,[1] Sergio O. Valenzuela,[3,4] and Igor Žutić[2]
[1] *Ioffe Institute, 194021 St. Petersburg, Russia*
[2] *Department of Physics, University at Buffalo, State University of New York, Buffalo, NY 14260, USA*
[3] *Catalan Institute of Nanoscience and Nanotechnology (ICN2), CSIC and BIST, Barcelona, Spain*
[4] *Institució Catalana de Recerca i Estudis Avançats (ICREA) Barcelona 08010, Spain*

## I. General Aspects of Spin and Pseudospin Resonances

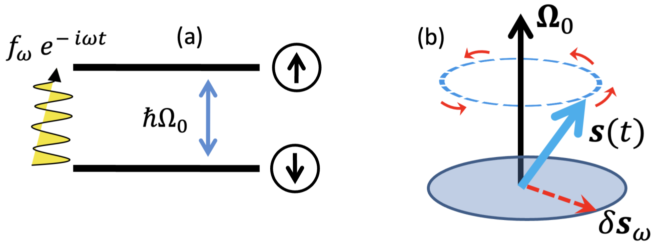


FIG. 1. Spin resonance from (a) quantum picture and (b) classical picture of spin precession. The parameters: $\boldsymbol{\Omega}_0 = \Omega_0 \hat{\boldsymbol{z}}$ is the Larmor frequency, $f_\omega e^{-i\omega t}$ is an oscillating external field, $\boldsymbol{s}(t)$ is the average spin and $\delta \boldsymbol{s}_\omega$ is the transverse spin component emerging due to $f_\omega$.

In this Section we summarize the basic elements of the spin resonance and describe its connection to the interband transitions for Dirac electrons. The Hamiltonian of a two-level system in an oscillating transverse field is given by

$$H = \hbar \Omega_0 s_z + \hbar \boldsymbol{f}(t) \boldsymbol{s}, \tag{1}$$

here the first term is responsible for the static Zeeman spin splitting, where $\boldsymbol{\Omega}_0 = \Omega_0 \hat{\boldsymbol{z}}$ is the Larmor precession frequency, while the second term describes an oscillating field inducing the spin resonance. The spin vector operator $\boldsymbol{s} = \boldsymbol{\sigma}/2$ and its $z$ component, $s_z$, consist of the Pauli matrices. In the second term, we assume the linear polarization $\boldsymbol{f}(t) = f(t)\hat{\boldsymbol{x}}$ with the oscillating field, $f(t) = f_\omega e^{-i\omega t} + \text{c.c.}$, where $\omega$ is the (angular) frequency. The corresponding matrix element of the time-dependent transition from the spin-down to the spin-up state, is given by

$$M_{\uparrow\downarrow} = \hbar \langle \uparrow | f_\omega s_x | \downarrow \rangle, \tag{2}$$

and the transition rate, $W_{\uparrow\downarrow}$, can be obtained from the Fermi's golden rule

$$W_{\uparrow\downarrow} = \frac{2\pi}{\hbar} |M_{\uparrow\downarrow}|^2 \delta(\hbar\omega - \Delta) = \frac{1}{2} \pi \hbar |f_\omega|^2 \delta(\hbar\omega - \Delta), \tag{3}$$

where $\Delta = \hbar\Omega_0$ is the spin splitting. The classical counterpart of this picture is based on the spin precession equation. The time-dependent average $\boldsymbol{s}(t) = \langle \boldsymbol{\sigma}/2 \rangle$ obeys the equation

$$\dot{\boldsymbol{s}} = [\boldsymbol{\Omega}_0 \times \boldsymbol{s}] + [\boldsymbol{f}(t) \times \boldsymbol{s}]\,. \tag{4}$$

To analyze $W_{\uparrow\downarrow}$ from the classical point of view, we employ the moving reference frame, $\hat{\boldsymbol{x}}' = \hat{\boldsymbol{\rho}}_+$ and $\hat{\boldsymbol{y}}' = (\hat{\boldsymbol{z}} \times \hat{\boldsymbol{\rho}}_+)$, rotating with the frequency $\boldsymbol{\omega} \parallel \hat{\boldsymbol{z}}$, here the ac-field is given by

$$\boldsymbol{f}(t) = \frac{f}{2} \left[ \hat{\boldsymbol{\rho}}_+(t) + \hat{\boldsymbol{\rho}}_-(t) \right], \tag{5}$$

$$\hat{\boldsymbol{\rho}}_\pm(t) = \hat{\boldsymbol{x}} \cos\omega t \pm \hat{\boldsymbol{y}} \sin\omega t. \tag{6}$$

Complementing Eq. (4) by a phenomenological damping rate $\gamma/\hbar$, in the rotating-wave approximation, the linear response of the transversal spin components $\boldsymbol{s}' = \hat{\boldsymbol{x}}' s'_x + \hat{\boldsymbol{y}}' s'_y$, is given by the static solution of

$$\dot{\boldsymbol{s}}' = [(\boldsymbol{\Omega}_0 - \boldsymbol{\omega}) \times \boldsymbol{s}'] + \frac{f}{2}\left[\hat{\boldsymbol{x}}' \times \boldsymbol{s}^0\right] - \hbar^{-1}\gamma \boldsymbol{s}', \tag{7}$$

with $\boldsymbol{s}^0 \parallel \boldsymbol{\Omega}_0$. $W_{\uparrow\downarrow}$ can be obtained by considering the evolution of the longitudinal spin component $W_{\uparrow\downarrow} = \dot{s}_z = [\boldsymbol{f}(t) \times \boldsymbol{s}']$. In the rotating reference frame this vector product is reduced to $\dot{s}_z = (f/2)s'_y$, with $s'_y$ given by

$$s'_y = \frac{1}{2}\frac{\hbar\gamma f/2}{(\hbar\omega - \Delta)^2 + \gamma^2}. \tag{8}$$

Recalling that $f = 2|f_\omega|$, we recover the Fermi's golden rule from Eq. (3)

$$W_{\uparrow\downarrow} = \frac{1}{2}\pi\hbar|f_\omega|^2 \frac{\gamma/\pi}{(\hbar\omega - \Delta)^2 + \gamma^2}, \tag{9}$$

where the delta-function is replaced by the Lorentzian.

The considered picture can be generalized to illustrate the interband absorption in graphene, or other two-dimensional (2D) hexagonal systems, where the low-energy effective Hamiltonian for an electron is constructed from the set of Pauli matrices of any physical origin. In case of a monolayer graphene in an oscillating electric field with $\boldsymbol{A}_\omega = (c/i\omega)\boldsymbol{E}_\omega$, for the $K$-valley we have

$$H = 2\hbar v_F \boldsymbol{\tau}\boldsymbol{k} - 2\frac{\hbar e}{c} v_F \boldsymbol{\tau}\boldsymbol{A}(t), \tag{10}$$

where $\boldsymbol{\tau} = \boldsymbol{\sigma}/2$ is the pseudospin vector originating from the presence of two inequivalent sublattices. It is straightforward to establish a correspondence of Eq. (10) with the Hamiltonian from Eq. (1) of an arbitrary two-level system, so that one could explicitly read out the effective static Zeeman field and the alternating field responsible for the pseudospin-flip transitions:

$$H = \hbar\boldsymbol{\Omega}_k \boldsymbol{\tau} + \hbar\boldsymbol{f}(t)\boldsymbol{\tau}, \tag{11}$$

where $\boldsymbol{\Omega}_k = 2v_F\boldsymbol{k}$ contains a subscript referring to the electron wave vector $\boldsymbol{k}$, and $\boldsymbol{f}(t) = -(2e/c)v_F\boldsymbol{A}(t)$.

In analogy with the spin resonance scheme, a quantum mechanical treatment of the absorption relies on the calculation of the matrix elements of optical transitions between eigenstates $|u_k^\pm\rangle$, corresponding to the static pseudospin vector $\boldsymbol{\tau}_k^\pm = \pm\hat{\boldsymbol{k}}/2$ co-aligned with $\boldsymbol{\Omega}_k$ and having opposite energies $\varepsilon_{k\pm} = \pm v_F k$. The matrix element is given by

$$M_k^{+-} = -2\frac{e}{c}v_F\langle u_k^+|(\boldsymbol{\tau}\boldsymbol{A}_\omega)|u_k^-\rangle, \tag{12}$$

and the absorption rate is obtained by summing the contribution of all electrons with the equilibrium distribution functions $f_{k,\pm}$

$$W = 4\frac{2\pi}{\hbar}\sum_k (f_{k-} - f_{k+})|M_k^{+-}|^2\delta(\hbar\omega - \hbar\Omega_k), \tag{13}$$

here, the factor 4 accounts for 2 valleys and 2 spin degrees of freedom in graphene. Performing the summation at zero temperature gives us the absorption coefficient $\alpha = (\pi e^2/\hbar c)\Theta(\hbar\omega - 2\mu)$, where $\mu$ is the Fermi energy and $\Theta$ is the Heaviside function. The classical picture corresponding to these transitions relies on the Bloch equations, which, in case of the Dirac Hamiltonian, take form

$$\dot{\boldsymbol{\tau}} = [\boldsymbol{\Omega}_k \times \boldsymbol{\tau}] + [\boldsymbol{f}(t) \times \boldsymbol{\tau}]\,. \tag{14}$$

The accurate treatment of these equations now requires one to take into account the geometry of the equilibrium pseudospin $\boldsymbol{\tau}_k^\pm$ and $\boldsymbol{\Omega}_k$, as well as its dependence on the electron wave vector $\boldsymbol{k}$, when summing over different electron states. The analysis and the derivation of the interband absorption coefficient based on the pseudospin resonance picture are presented in detail in the following Sections of this Supplemental Material.

## II. Spin Resonance Absorption From the Kubo Formula

We use the Kubo formula [1, 2] for the ac-conductivity at (angular) frequency, $\omega$

$$\sigma_{\alpha\beta}(\omega) = -\frac{i\hbar e^2}{S}\sum_{k,\nu\nu'}\frac{f_{k,\nu}-f_{k,\nu'}}{\varepsilon_{k,\nu}-\varepsilon_{k,\nu'}}\frac{\boldsymbol{v}^{\alpha}_{k\nu;k\nu'}\boldsymbol{v}^{\beta}_{k\nu';k\nu}}{\varepsilon_{k,\nu}-\varepsilon_{k,\nu'}+\hbar\omega+i0}, \tag{15}$$

where $f_{k,\nu}$ is the equilibrium distribution function of electrons in the state with energy $\varepsilon_{k,\nu}$,. The index $\nu$ denotes pseudospin, spin and valley degrees of freedom, and $S$ is the area of the sample. $\boldsymbol{v}^{\alpha,\beta}_{k\nu;k\nu'}$ are the proper matrix elements, with $\alpha, \beta = x, y$, of the velocity operator $\boldsymbol{v} = \partial\mathcal{H}/\partial\boldsymbol{p}$, where $\mathcal{H}$ is the Hamiltonian and $\boldsymbol{p} = \hbar\boldsymbol{k}$ is the momentum. The absorption coefficient for the linearly polarized electric field, $E_x$, and $\nu \neq \nu'$ is

$$\alpha(\omega) = \frac{4\pi}{c}\mathrm{Re}\left[\sigma_{xx}(\omega)\right] = \frac{4\pi}{c}\frac{\pi e^2}{\omega S}\sum_{k,\nu\neq\nu'}\left(f_{k,\nu}-f_{k,\nu'}\right)\left|v^{x}_{\nu\nu'}(\boldsymbol{k})\right|^2\delta\left(\varepsilon_{k,\nu}-\varepsilon_{k,\nu'}+\hbar\omega\right). \tag{16}$$

We consider $n$-doped, proximity-modified, monolayer graphene layer described by the Hamiltonian

$$\mathcal{H} = 2v_F(\xi\tau_x p_x + \tau_y p_y) + (\boldsymbol{\Delta}\cdot\boldsymbol{s}) + 2\lambda_{\mathrm{so}}\left(\xi\tau_x s_y - \tau_y s_x\right), \tag{17}$$

where, as before, $\boldsymbol{\tau}$ and $\boldsymbol{s}$ are the pseudospin and spin vectors, $\xi = \pm 1$ for $(K, K')$ valleys, $\boldsymbol{\Delta}$ is the proximity-induced magnetic exchange field, while the last term represents the spin-orbit coupling (SOC), described by its strength $\lambda_{\mathrm{so}}$, to be treated perturbatively, as discussed in the main text. By neglecting the SOC, the band structure and its eigenstates are given by

$$\varepsilon^{\pm}_{k,s} = \pm v_F p + s\Delta, \qquad s = \pm\frac{1}{2}, \tag{18}$$

$$(\boldsymbol{\Delta}\cdot\boldsymbol{s})\ |s\rangle = s\Delta\ |s\rangle, \tag{19}$$

$$|u^{\pm}_{k,s}\rangle = \frac{1}{\sqrt{2}}\begin{pmatrix}1\\ \pm\xi e^{i\xi\varphi}\end{pmatrix}|s\rangle. \tag{20}$$

We focus on the spin-flip direct intersubband transitions in the conduction band $(k,+,\downarrow) \to (k,+,\uparrow)$. For the eigenstates from Eq. (20), the matrix element $v^{\alpha}_{(k,+,\uparrow);(k,+,\downarrow)} = 0$ is absent as the two spin states $|\uparrow\rangle, |\downarrow\rangle$ are orthogonal. To get the spin-flip transitions, one needs to take into account SOC-induced corrections to the wave functions. In the linear order with respect to SOC, the matrix elements of $\hat{\boldsymbol{v}} = 2v_F(\xi\tau_x, \tau_y)$ for the considered transition are given by

$$v^{\alpha}_{\uparrow\downarrow} = -\frac{iv_F\lambda_{\mathrm{so}}(pv_F)}{\Delta^2-(2pv_F)^2}\mathcal{Q}_{\alpha}(\varphi), \tag{21}$$

where $\mathcal{Q}_{\alpha}(\varphi)$ describes the angular dependence. The explicit expressions for $\mathcal{Q}_{\alpha}(\varphi)$ are summarized in the Table I.

| Exchange \ Polarization | $(x)$ | $(y)$ | $(+)$ | $(-)$ |
|---|---|---|---|---|
| $\boldsymbol{\Delta} \parallel \hat{\boldsymbol{z}}$ | $e^{-2i\varphi}-1$ | $i(1+e^{-2i\varphi})$ | $\sqrt{2}$ | $\sqrt{2}e^{-2i\varphi}$ |
| $\boldsymbol{\Delta} \parallel \hat{\boldsymbol{x}}$ | $2\sin^2\varphi$ | $-\sin 2\varphi$ | $i\sqrt{2}e^{i\varphi}\sin\varphi$ | $i\sqrt{2}e^{-i\varphi}\sin\varphi$ |

TABLE I. Angular dependence of $\mathcal{Q}_{\alpha}(\varphi)$ for the out-of-plane and in-plane orientations of $\boldsymbol{\Delta}$, and different polarizations of $\boldsymbol{E}_{\omega}$, here $(x, y)$ corresponds to the linear polarization along the $\hat{\boldsymbol{x}}, \hat{\boldsymbol{y}}$ axes, respectively, and $(\pm)$ describes the circular polarization (helicity).

Here $\alpha = (\pm)$ corresponds to the circular polarization velocity operator determined as $v^{\pm}_{\uparrow\downarrow} = (v^{x}_{\uparrow\downarrow} \pm iv^{y}_{\uparrow\downarrow})/\sqrt{2}$. The matrix elements are identical for $(K, K')$ valleys (up to some phase factor). By substituting $v^{\alpha}_{\uparrow\downarrow}(\boldsymbol{k})$ in Eq. (16), we express the absorption coefficient at $T = 0$ K as

$$\alpha_{\mathrm{sf}}(\omega) = 8\pi\frac{e^2}{\hbar c}\frac{\lambda^2_{\mathrm{so}}}{\Delta}b\mathcal{I}\delta(\hbar\omega-\Delta), \qquad \mathcal{I} = \int\limits_{\mu-\Delta/2}^{\mu+\Delta/2}\frac{x^3dx}{[(2x)^2-\Delta^2]^2}, \tag{22}$$

where $b$ accounts for averaging of $|v^{\alpha}_{\uparrow\downarrow}(\boldsymbol{k})|^2$ over momentum directions and it is discussed in the main text. A straightforward evaluation of the integral gives

$$\alpha_{\rm sf}(\omega) = \pi \frac{e^2}{\hbar c} b \frac{\lambda_{\rm so}^2}{4\Delta} \left[ \ln\left(\frac{\mu+\Delta}{\mu-\Delta}\right) + \frac{\Delta^3/2\mu}{(\mu^2-\Delta^2)} \right] \delta(\hbar\omega - \Delta), \tag{23}$$

where, as before, $\mu$ is the Fermi energy. The analysis of this expression shows that, at $\mu \gtrsim 2\Delta$, the coefficient is approximately given by

$$\alpha_{\rm sf}(\omega) = \pi \frac{e^2}{\hbar c} \frac{\lambda_{\rm so}^2}{2\mu} \delta(\hbar\omega - \Delta). \tag{24}$$

We note that in the main text we replace the exact delta-function by a Lorentzian broadening line with a spin dephasing rate, $\gamma$.

### III. Spin Resonance Absorption From the Mean-Field Theory

As given in the main text, we write the total electron Hamiltonian in the form

$$\mathcal{H} = \hbar \boldsymbol{\Omega}_k \cdot \boldsymbol{\tau} + \hbar \boldsymbol{\Omega}_{\rm ex} \cdot \boldsymbol{s} + \hbar \boldsymbol{\Omega}_{\rm so}(\boldsymbol{\tau}) \cdot \boldsymbol{s} + \hbar \boldsymbol{\Omega}_{\rm int}(t) \cdot \boldsymbol{\tau}, \tag{25}$$

where the first term defines the Dirac spectrum, the second is the magnetic exchange, $\boldsymbol{\Delta} = \hbar\boldsymbol{\Omega}_{\rm ex}$, the third gives SOC, while the last term describes the electron pseudospin coupling to an external ac-electric field, $\boldsymbol{\Omega}_{\rm int} = -2(e/\hbar c) v_F (\xi A_x, A_y)$, via vector potential, $\boldsymbol{A}_\omega$. For an electron with $\boldsymbol{k}$, the equations of motion of its spin $\boldsymbol{s}(t)$ and pseudospin $\boldsymbol{\tau}(t)$ in the mean-field approximation are given by

$$\dot{\boldsymbol{\tau}} = \left[ (\boldsymbol{\Omega}_k + \boldsymbol{\Omega}'_{\rm so}(\boldsymbol{s})) \times \boldsymbol{\tau} \right] + \left[ \boldsymbol{\Omega}_{\rm int}(t) \times \boldsymbol{\tau} \right], \tag{26}$$

$$\dot{\boldsymbol{s}} = \left[ (\boldsymbol{\Omega}_{\rm ex} + \boldsymbol{\Omega}_{\rm so}(\boldsymbol{\tau})) \times \boldsymbol{s} \right], \tag{27}$$

where $\boldsymbol{\Omega}'_{\rm so}(\boldsymbol{s})$ can be obtained by considering $\boldsymbol{\tau} \cdot \boldsymbol{\Omega}'_{\rm so}(\boldsymbol{s}) = \boldsymbol{s} \cdot \boldsymbol{\Omega}_{\rm so}(\boldsymbol{\tau})$. We further analyze these equations for the model considered in the second section and for the perpendicular (out-of-plane) orientation of the magnetic exchange field, $\boldsymbol{\Delta} = \Delta \hat{\boldsymbol{z}}$. In equilibrium, a $K$-valley electron with $\boldsymbol{k}$ has its pseudospin $\boldsymbol{\tau}^0$ parallel to $\boldsymbol{\Omega}_k = 2 v_F k \hat{\boldsymbol{k}}$ (ignoring weak SOC). Applying $\boldsymbol{\Omega}_{\rm int}(t) \propto \boldsymbol{A}_\omega e^{-i\omega t}$ leads to the appearance of the torque $\left[ \boldsymbol{\Omega}_{\rm int} \times \boldsymbol{\tau}^0 \right]$ acting on the pseudospin and generating the linear response correction, $\delta\boldsymbol{\tau}_\omega = \delta\tau_z \hat{\boldsymbol{z}} + \delta\tau_\varphi \hat{\boldsymbol{\varphi}}$, given by

$$\delta\tau_{z,\varphi}(\omega) = \tau^0 \frac{\alpha_{z,\varphi} 2\mathcal{T}}{\Omega_k^2 - \omega^2}, \qquad \mathcal{T} = e \frac{v_F}{\hbar c} [\boldsymbol{A}_\omega \times \hat{\boldsymbol{k}}]_z, \tag{28}$$

where $\alpha_{z,\varphi} = (-i\omega, \Omega_k)$ and $\tau^0 = \pm 1/2$ corresponds to conduction and valence bands, respectively. This expression displays the pseudospin resonance at the frequency $\omega = \Omega_k$, which corresponds to the spin-conserving interband absorption. Having found $\delta\boldsymbol{\tau}_\omega$, we can calculate the interband absorption coefficient from the real part of the optical conductivity as follows

$${\rm Re}[j_x(\omega)] = e \sum_{k, s=\pm 1/2} {\rm Re}\left[ 2 v_F \delta\tau^s_\varphi(\omega) (\hat{\boldsymbol{\varphi}} \cdot \hat{\boldsymbol{x}}) \right] (f_{k,-,s} - f_{k,+,s}), \tag{29}$$

here $j_x(\omega)$ is the electric current density. Performing this summation we arrive at the expression for the absorption coefficient in form $\alpha = (\pi e^2/2\hbar c)(\Theta[\hbar\omega - 2\mu + \Delta] + \Theta[\hbar\omega - 2\mu - \Delta])$.

The oscillating pseudospin plays the role of an external ac-field acting on the electron spin in Eq. (26) via spin-orbital field, $\hbar\boldsymbol{\Omega}_{\rm so}(t) = 2\lambda_{\rm so}[\hat{\boldsymbol{z}} \times \delta\boldsymbol{\tau}(t)] = -2\lambda_{\rm so}\delta\tau_\varphi(t)\hat{\boldsymbol{k}}$, where $\delta\boldsymbol{\tau}(t) = 2{\rm Re}[e^{-i\omega t}\delta\boldsymbol{\tau}_\omega]$. The SOC field appears in the linear polarization (along $\hat{\boldsymbol{k}}$) and it is determined by the single component $\delta\tau_\varphi$. In the out-of-plane geometry, $\boldsymbol{s}^0 \parallel \boldsymbol{\Delta} \parallel \hat{\boldsymbol{z}}$, we get for the linear spin response, $\delta\boldsymbol{s}_\omega = \delta s_k \hat{\boldsymbol{k}} + \delta s_\varphi \hat{\boldsymbol{\varphi}}$,

$$\delta s_{k,\varphi}(\omega) = s^0 \frac{\beta_{k,\varphi}}{\Omega_{\rm ex}^2 - \omega^2} 2\lambda_{\rm so} \delta\tau_\varphi(\omega) = s^0 \tau^0 \frac{2\lambda_{\rm so}\beta_{k,\varphi}\Omega_k 2\mathcal{T}}{(\Omega_{\rm ex}^2 - \omega^2)(\Omega_k^2 - \omega^2)}, \tag{30}$$

where $\beta_{k,\varphi} = (\Omega_{\rm ex}, -i\omega)$ and $s^0 = \pm 1/2$ corresponds to $|\uparrow\rangle, |\downarrow\rangle$ spin states. This expression is presented in the main text. To analyze the energy absorption due to the spin resonance, we write the SOC-field as

$$\boldsymbol{\Omega}_{\rm so}(t) = \frac{\Omega_{\rm so}}{2} \left[ \hat{\boldsymbol{\rho}}_+(t) + \hat{\boldsymbol{\rho}}_-(t) \right], \tag{31}$$

where $\Omega_{\rm so} = -2\lambda_{\rm so}|\delta\tau_\varphi|$, and $\hat{\boldsymbol{\rho}}_\pm(t)$ is given in Eq. 6. We shift to the rotating frame, $\hat{\boldsymbol{x}}' = \hat{\boldsymbol{\rho}}_+$ and $\hat{\boldsymbol{y}}' = (\hat{\boldsymbol{z}} \times \hat{\boldsymbol{\rho}}_+)$; in the rotating wave approximation the emerging spin $\boldsymbol{s}' = \hat{\boldsymbol{x}}' s'_x + \hat{\boldsymbol{y}}' s'_y$, is found from

$$\frac{d\boldsymbol{s}'}{dt} = [(\boldsymbol{\Omega}_{\rm ex} - \boldsymbol{\omega}) \times \boldsymbol{s}'] + \frac{\Omega_{\rm so}}{2}\left[\hat{\boldsymbol{x}}' \times \boldsymbol{s}^0\right] - \hbar^{-1}\gamma \boldsymbol{s}', \tag{32}$$

where we introduced the phenomenological spin relaxation rate of the transverse components, $\gamma \to 0$. The steady-state solution for $s'_y$ is

$$s'_y = \frac{1}{2}\frac{\gamma(-\hbar\Omega_{\rm so}s^0)}{(\hbar\omega - \Delta)^2 + \gamma^2}. \tag{33}$$

The transition rate is given by

$$W_k = -\frac{1}{2}\Omega_{\rm so}s'_y = \frac{\pi}{\hbar}s^0\lambda_{\rm so}^2|\delta\tau_\varphi|^2\mathcal{L}(\hbar\omega), \qquad \mathcal{L}(\hbar\omega) = \frac{\gamma/\pi}{(\hbar\omega - \Delta)^2 + \gamma^2}. \tag{34}$$

For the linear polarization, $\boldsymbol{A}_\omega \parallel \hat{\boldsymbol{x}}$, we have $|\delta\tau_\varphi| = 2|\delta\tau_\varphi(\omega)|$ and $|\delta\tau_\varphi(\omega)|^2 \propto [\hat{\boldsymbol{x}} \times \hat{\boldsymbol{k}}]_z^2 = \sin^2\varphi$, which yields

$$W_k = s^0\frac{16\pi}{\hbar}\left[\frac{\lambda_{\rm so}v_F p\sin\varphi}{\Delta^2 - (2pv_F)^2}\frac{e}{c}v_F A_\omega\right]^2\mathcal{L}(\hbar\omega), \tag{35}$$

here we took into account that $W_k$ is nonzero in a narrow region $\hbar\omega \approx \Delta$, thus we replaced $\hbar\omega \to \Delta$ in a nonresonant prefactor. One can compare this expression with the matrix elements of the velocity operator calculated in Eq. (21). To calculate the absorption coefficient, we further need to sum over $\boldsymbol{k}$-electrons with the distribution function $f_{k,s}$, which gives

$$\alpha_{\rm sf}(\omega) = 2\frac{\hbar\omega}{I_\omega}\sum_k (f_{k\uparrow} - f_{k\downarrow})\,|W_k|, \tag{36}$$

where 2 accounts for $K, K'$ valleys and $I_\omega = \omega^2|A_\omega|^2/2\pi c$. A straightforward calculation of this expression gives the formula for the absorption coefficient in form of Eq. (22), derived by the Kubo formalism.

## IV. Massive Dirac Electrons

In this section we consider the EDSR for massive Dirac electrons with the mass term arising from a staggered potential of strength $U \equiv \hbar\Omega_{\rm g}$. The Hamiltonian is given by

$$\mathcal{H} = \hbar\boldsymbol{\Omega}_k\cdot\boldsymbol{\tau} + \hbar\boldsymbol{\Omega}_{\rm ex}\cdot\boldsymbol{s} + \hbar\boldsymbol{\Omega}_{\rm so}(\boldsymbol{\tau})\cdot\boldsymbol{s} + \hbar\boldsymbol{\Omega}_{\rm int}(t)\cdot\boldsymbol{\tau}, \tag{37}$$

but now the Larmor frequency $\boldsymbol{\Omega}_k$ for the pseudospin contains the massive term due to a staggered potential

$$\boldsymbol{\Omega}_k = 2v_F(\xi k_x, k_y, \Omega_{\rm g}/2v_F), \qquad \Omega_k = \sqrt{\Omega_{\rm g}^2 + (2v_F k)^2}. \tag{38}$$

Without SOC, the spectrum and the eigenfunctions are given by

$$\varepsilon^\pm_{k,s} = \pm\frac{1}{2}\hbar\Omega_k + s\Delta, \qquad s = \pm\frac{1}{2}, \tag{39}$$

$$(\boldsymbol{\Delta}\cdot\boldsymbol{s})\;|s\rangle = s\Delta\;|s\rangle, \tag{40}$$

$$|u^\pm_{k,s}\rangle = \frac{1}{\sqrt{2}}\begin{pmatrix} a^\pm_k \\ \pm\xi a^\mp_k e^{i\xi\varphi}\end{pmatrix}|s\rangle, \tag{41}$$

where $a^\pm_k = \sqrt{1 \pm \Omega_{\rm g}/\Omega_k}$. We next consider the regime with $U > \Delta$, and the Fermi energy $\mu > U/2 - \Delta/2$ corresponding to the $n$-doping (see the spectrum in Fig.4b of the main text). To calculate the absorption coefficient we follow the procedure from the first and second sections of this Supplemental Material. Below we present the details for the $\boldsymbol{\Delta} \parallel \hat{\boldsymbol{z}}$ geometry. In the first order with respect to $\lambda_{\rm so}$, we get for the matrix elements of $\hat{\boldsymbol{v}} = 2v_F(\xi\tau_x, \tau_y)$

$$v^x_{\uparrow\downarrow} = 2i\eta \frac{\Omega_{\rm g}(\Omega_{\rm ex}-\Omega_{\rm g}) + (v_F k)^2(e^{2i\varphi}-1)}{\Omega_k\left(\Omega_{\rm ex}^2 - 4\Omega_k^2\right)}, \tag{42}$$

$$v^+_{\uparrow\downarrow} = \eta \frac{\Omega_{\rm g}^2 + \xi\Omega_{\rm g}\Omega_{\rm ex} + 2(v_F k)^2}{\Omega_k(\Omega_k^2 - \Omega_{\rm ex}^2)}, \qquad v^-_{\uparrow\downarrow} = \eta\frac{2e^{-2i\varphi}(v_F k)^2}{\Omega_k(\Omega_k^2-\Omega_{\rm ex}^2)}, \tag{43}$$

where the prefactor $\eta = i\sqrt{2}\lambda_{\rm so} v_F/\hbar$. We note that $v^+_{\uparrow\downarrow}$ depends on the valley index $\xi = \pm 1$. To calculate the absorption coefficient, $\alpha_{\rm sf}$, presented in Figs. 3 and 4 of the main text we substitute this expression in Eq. (16) and evaluate the integral numerically [similar to Eq. (22)].

Let us analyze the polarization dependence of $\alpha_{\rm sf}$ from Figs. 3 and 4, discussed also in the main text. For $v_F k \to 0$ we get $\alpha^+_{\rm sf} \gg \alpha^-_{\rm sf}$, which indicates a recovered polarization selectivity of the EDSR. At the same moment, the EDSR absorption at $\sigma^+$ is slightly different for $K$ and $K'$ valleys. These features can be seen from the velocity matrix elements in Eq. (43), here $v^-_{\uparrow\downarrow} \propto (v_F k)^2 \to 0$, while $v^+_{\uparrow\downarrow} \propto \Omega_{\rm g}^2 + \xi\Omega_{\rm g}\Omega_{\rm ex} \neq 0$ remains finite and depends on $\xi$. It is instructive to understand this behavior based on the coupled spin-pseudospin dynamics.

Ignoring the role of SOC for the pseudospin dynamics, we note that the eigen pseudospin vector $\boldsymbol{\tau}^0 = \langle u^+_{k,s}|\hat{\boldsymbol{\tau}}|u^+_{k,s}\rangle$ is directed along the overall Larmor frequency $\boldsymbol{\tau}^0 \parallel \boldsymbol{\Omega}_k$ and in case of finite mass term $U \neq 0$ has a nonzero component along $\hat{\boldsymbol{z}}$ direction, i.e. $\tau^0_z = \Omega_{\rm g}/2\Omega_k$, which approaches $\tau^0_z \to 1/2$ close to the conduction band bottom, $v_F k \ll \Omega_{\rm g}$.

We expand related discussion by considering the EDSR for both $K, K'$ valleys on equal footing and focus on the circular polarization of the incident wave. The pseudospin dynamics is induced by external ac-electric field via $\boldsymbol{\Omega}_{\rm int} = -2(e/\hbar c)v_F(\xi A_x, A_y)$. For circularly polarized vector potential $\boldsymbol{A}(t) = A\hat{\boldsymbol{\rho}}_\sigma(t)$, where $\hat{\boldsymbol{\rho}}_\sigma(t)$ is the unit vector rotating counter- and clockwise, respectively [see Eq. (31)], we give $\boldsymbol{\Omega}^\sigma_{\rm int}(t) = \Omega_{\rm int}\hat{\boldsymbol{\rho}}_{\xi,\sigma}(t)$, where $\Omega_{\rm int} = -2(e/\hbar c)v_F A$ and the vector $\hat{\boldsymbol{\rho}}_{\xi,\sigma}(t)$ includes the dependence on the valley index, $\hat{\boldsymbol{\rho}}_{\xi,\sigma}(t) = \xi\hat{\boldsymbol{x}}\cos\omega t + \sigma\hat{\boldsymbol{y}}\sin\omega t$. The Fourier components of this field $\boldsymbol{\Omega}_{\omega,{\rm int}}e^{-i\omega t} = \Omega_{\rm int}\hat{\boldsymbol{\rho}}_{\xi,\sigma}e^{-i\omega t}$, where $\hat{\boldsymbol{\rho}}_{\xi,\sigma} = (\xi\hat{\boldsymbol{x}} + i\sigma\hat{\boldsymbol{y}})/2$, gives rise to $\delta\boldsymbol{\tau}_\omega e^{-i\omega t}$, that can be found from Eq. (26)

$$-i\omega\delta\boldsymbol{\tau}_\omega = \Omega_{\rm g}\left[\hat{\boldsymbol{z}}\times\delta\boldsymbol{\tau}_\omega\right] + \Omega_{\rm int}\left[\hat{\boldsymbol{\rho}}_{\xi,\sigma}\times\boldsymbol{\tau}^0\right]. \tag{44}$$

The pseudospin vector $\delta\boldsymbol{\tau}_\omega = \hat{\boldsymbol{x}}\delta\tau_{\omega\,x} + \hat{\boldsymbol{y}}\delta\tau_{\omega\,y}$ is thus given by

$$\begin{pmatrix}\delta\tau_{\omega\,x}\\ \delta\tau_{\omega\,y}\end{pmatrix} = \frac{1}{2}\tau_0\frac{\Omega_{\rm int}}{\Omega_{\rm g}^2-\omega^2}\begin{pmatrix}\sigma\omega + \xi\Omega_{\rm g}\\ i\sigma\Omega_{\rm g} + i\xi\omega\end{pmatrix}. \tag{45}$$

Close to the pseudospin resonance frequency, $\omega = \Omega_{\rm g} = U/\hbar$, the vector $\delta\boldsymbol{\tau}_\omega$ is finite only provided that $\sigma = \xi$, which sets the optical absorption selection rules for the interband transitions (in the spin conserving channels). The pseudospin resonance in $K$ and $K'$ valleys occurs for $\sigma^+$ and $\sigma^-$ polarization, respectively, displaying the well-known valley-sensitive circular dichroism of gapped Dirac electrons [3]. In terms of the pseudospin resonance, the direction of the rotation of $\boldsymbol{\Omega}_{\rm int}(t) \parallel \hat{\boldsymbol{\rho}}_{\xi,\sigma}(t)$ depends on $\xi = \pm 1$ and is opposite for $K, K'$ valleys.

In our model the EDSR takes place at $\omega = \Omega_{\rm ex} < \Omega_{\rm g}$. Going away from the pseudospin resonance we recover nonzero $\delta\boldsymbol{\tau}_\omega$ for both circular polarizations. In the limit $\Omega_{\rm g} \gg \omega \sim \Omega_{\rm ex}$ we keep only $U$-related terms in the Eq. (45) and get

$$\delta\boldsymbol{\tau}(t) = 2{\rm Re}\left[e^{-i\omega t}\delta\boldsymbol{\tau}_\omega\right] = \tau_0\frac{\Omega_{\rm int}\Omega_{\rm g}}{\Omega_{\rm g}^2-\omega^2}\hat{\boldsymbol{\rho}}_{\xi,\sigma}(t). \tag{46}$$

The spin dynamics in the mean-field approximation is govern by the Eq. (27)

$$\delta\dot{\boldsymbol{s}} = \left[\boldsymbol{\Omega}_{\rm ex}\times\delta\boldsymbol{s}\right] + \left[\boldsymbol{\Omega}_{\rm so}(t)\times\boldsymbol{s}^0\right], \tag{47}$$

with the SOC field $\boldsymbol{\Omega}_{\rm so}(t) = 2\lambda_{\rm so}(-\delta\tau_y, \xi\delta\tau_x)$. Substituting $\delta\boldsymbol{\tau}(t)$ from Eq. (46), we get for $\tau^0 = 1/2$

$$\boldsymbol{\Omega}_{\rm so}(t) = \lambda_{\rm so}\frac{\Omega_{\rm int}\Omega_{\rm g}}{\Omega_{\rm g}^2-\omega^2}\left[\hat{\boldsymbol{z}}\times\hat{\boldsymbol{\rho}}_\sigma(t)\right]. \tag{48}$$

It is important to note that $\boldsymbol{\Omega}_{\rm so}$ does not depend on the valley index $\xi$ and lies entirely in the plane of the electron motion. At the same time, the direction of the rotation of the vector $[\hat{\boldsymbol{z}}\times\hat{\boldsymbol{\rho}}_\sigma(t)]$ coincides with $\hat{\boldsymbol{\rho}}_\sigma(t)$. Therefore, the spin resonance for $\delta\boldsymbol{s}(t)$ will obey the regular polarization rules, independent of the valley, i.e. at $\boldsymbol{\Omega}_{\rm ex} \parallel \hat{\boldsymbol{z}}$, the EDSR absorption will be active uniquely for $\hat{\boldsymbol{\rho}}_+$ polarization for both valleys.

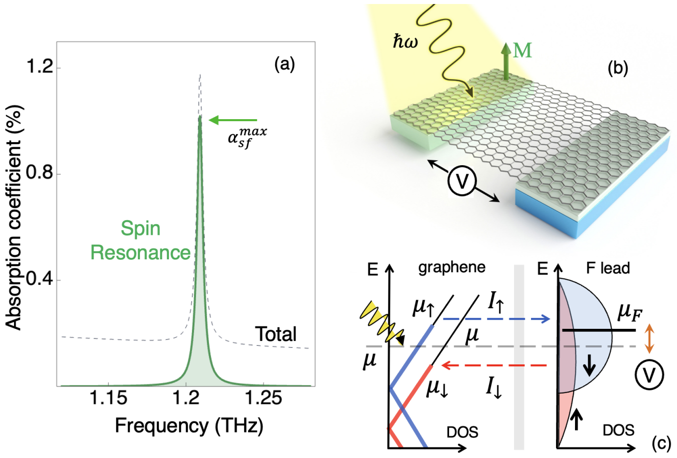


FIG. 2. (a): The absorption, $\alpha(\omega)$, near the spin resonance. Solid line: purely EDSR $\alpha_{\rm sf}(\omega)$, the dotted line: a total $\alpha(\omega)$ with the Drude absorption tail. The parameters are $\Delta = 5$ meV, $f_0 \approx 1.2$ THz, $\mu = 16$ meV, $\hbar/\gamma = 70$ ps, and $\tau_p = 6.5$ ps. (b): Scheme of the electrical spin detection. Photogenerated spin polarization in graphene leads to the electromotive force, EMF, and the associated voltage, $V$, at the graphene-ferromagnet interface upon THz radiation. The density of states (DOS) is spin dependent.

A weak valley dependence at small $\mu$ obtained in the numerical calculation and seen in the velocity matrix elements of Eq. (43) is reflected in the coupled spin-pseudospin dynamics when accounting both for $\omega$ and $U$ in Eq. (45), the latter gives the dependence on the valley index. The absorption coefficient corresponding to the EDSR can be obtained by the similar procedure discussed in the previous Section. The dependence of $\alpha_{\rm sf}^{\rm max}$ on $\mu$ is shown in Fig. 4 in the main text. The presence of the polarization selectivity at small $\mu$ is a consequence of the discussed underlying geometry in the coupled spin-pseudospin dynamics. Increasing $\mu$ will strongly modify the polarization selection rules, such that at $\mu \gg U$, we recover the expression $\alpha_{\rm sf}(\omega) = \alpha_0 \lambda_{\rm so}^2/(2\pi\mu\gamma)$ for the absorption coefficient that is polarization independent and which coincides with the absorption for the linear spectrum.

## V. Electrical Detection of the EDSR

A strong spin resonance, depicted in Fig. 2(a), accompanying the EDSR response of a proximitized graphene, could be detected electrically in a scheme depicted in Fig. 2(b). For an experimental implementation, it is important to largely retain properties of a pristine graphene, which can be readily realized not only with ferromagnetic insulators, but also with ferromagnetic metals [4, 5]. Importantly, the magnetic proximity effect remains essential in this setting leading to the Dirac cones spin splitting and to the bias-controlled graphene doping [4]. The latter suggests that the graphene layer and ferromagnet (F) share the common Fermi level at their contact, allowing for the electron transfer across the interface. Because of the spin-dependent tunneling into F contact, the photogenerated nonequilibrium spin polarization in graphene leads to the appearance of an electromotive force (EMF) at the graphene/F interface, which can be detected electrically using Johnson-Silsbee scheme [6].

The emerging EMF voltage $V$ can be estimated as follows. The current $I_{\uparrow,\downarrow}$ of spin-up and spin-down electrons across the interface is given by $I_{\uparrow,\downarrow} = G_{\uparrow,\downarrow}(\mu_{\uparrow,\downarrow} - \mu_F)$, where $e^2 G_{\uparrow,\downarrow}$ is the spin-dependent conductance of the graphene/F interface, the nonequilibrium chemical potentials $\mu_{\uparrow,\downarrow}$ differ for spin states in graphene while $\mu_F$ remains spin-independent in F assuming fast equilibration in the lead, see Fig. 2. We introduce $\mu = (\mu_\uparrow + \mu_\downarrow)/2$ and $\mu_s = (\mu_\uparrow - \mu_\downarrow)/2$. The EMF voltage $V$ corresponds to $V = (\mu_F - \mu)/e$. In the steady-state regime, no electric current flows, $I_\uparrow + I_\downarrow = 0$ and we get $V = (G_s/eG)\mu_s$, where $G_s = (G_\uparrow - G_\downarrow)$ and $G = G_\uparrow + G_\downarrow$. The spin current is then $I_s = G\mu_s - G_s eV$. The spin relaxation term can be expressed as $S - S_0 \approx \langle g \rangle \mu_s$ with $\langle g \rangle$ being the average density of states for given $\mu$. Collecting all the terms we obtain

$$V = e^{-1}\eta W_s T_*, \quad T_*^{-1} = 2\frac{G_\uparrow G_\downarrow}{G} + \frac{\langle g \rangle}{\tau_s}, \tag{49}$$

where $\eta = G_s/G$ is the spin transparency of the interface and $T_*$ is an overall spin relaxation time.

To estimate the magnitude of $V$ upon steady radiation, we assume $T_*^{-1} \approx G$, at that $V \approx G^{-1}\eta W_s/e$ with $W_s \approx \alpha_{\rm sf}^{\max} P_\omega/(\hbar\omega)$, where $P_\omega$ is the radiation power. Taking $\alpha_{\rm sf}^{\max} \approx 0.5\alpha_0$ for $\hbar\omega = 5$ meV, $P_\omega = 10^{-2}$ W, $G^{-1} \approx 2.5\Omega$ and $\eta = 10\%$ we get $V \approx 2$ mV. This suggests the responsivity of 0.2 V/W, comparable with the state of the art graphene THz detectors [7].

* denisokonstantin@gmail.com

[1] S. Barati and S. H. Abedinpour, "Optical conductivity of three and two dimensional topological nodal-line semimetals," Phys. Rev. B **96**, 155150 (2017).

[2] K. Nomura and A. H. MacDonald, "Quantum transport of massless dirac fermions," Phys. Rev. Lett. **98**, 076602 (2007).

[3] D. Xiao, G. Liu, W. Feng, X. Xu, and W. Yao, "Coupled Spin and Valley Physics in Monolayers of $MoS_2$ and Other Group-VI Dichalcogenides," Phys. Rev. Lett. **108**, 196802 (2012).

[4] P. U. Asshoff, J. L. Sambricio, A. P. Rooney, S. Slizovskiy, A. Mishchenko, A. M. Rakowski, E. W. Hill, A. K. Geim, S. J. Haigh, V. I. Fal'Ko, I. J. Vera-Marun, and I. V. Grigorieva, "Magnetoresistance of vertical Co-graphene-NiFe junctions controlled by charge transfer and proximity-induced spin splitting in graphene," 2D Mater. **4**, 031004 (2017).

[5] J. Xu, S. Singh, J. Katoch, G. Wu, T. Zhu, I. Žutić, and R. K. Kawakami, "Spin inversion in graphene spin valves by gate-tunable magnetic proximity effect at one-dimensional contacts," Nat. Commun. **9**, 2869 (2018).

[6] J. Fabian, A. Matos-Abiague, C. Ertler, P. Stano, and I. Žutić, "Semiconductor spintronics," Acta Phys. Slovaca **57**, 565 (2007).

[7] J. Liu, X. Li, R. Jiang, K. Yang, J. Zhao, S. A. K., J. He, P. Liu, J. Zhu, and B. Zeng, "Recent progress in the development of graphene detector for terahertz detection," Sensors **21**, 4987 (2021).
